# Supplementary material for: Frequency Throttling Side-Channel Attack
Source: arXiv:2206.07012 source file (2023-05-24)
Supplement: Supplementary file 1 [file Appendix.tex]

\section{Appendix} \label{sec:appendix}
In this section, we list the revisions we have made:
